# Supplementary material for: Near-Optimal Multi-Agent Learning for Safe Coverage Control
Source: arXiv:2210.06380 source file (2022-10-12)
Supplement: Supplementary file 1 [file H-information-gain.tex]

\section{Definition of information gain and bound on it}
For \textbf{selecting a point corresponding to maximum $\sigma$(x)$\to \LocAgent[m,i]{t}$} among $\Discat[i-]_t$ points in round t by agent i for T rounds,

\begin{align*}
    I(Y_{\LocAgent[m,1:\numOfAgents]{1:T}};\density) &= H(Y_{\LocAgent[m,1:\numOfAgents]{1:T}}) - H(Y_{\LocAgent[m,1:\numOfAgents]{1:T}}|\density) \numberthis \label{eqn: max-single-total-info}
\end{align*}

Now consider, the observation of the $\numOfAgents$ agents at time t. To generalize it to constraint case, let say we don't receive \numOfAgents measurements at all times but $\numOfAgents'_t \leq \numOfAgents$. For agent i, observation at $\LocAgent[m, i]{t}$ is $\{ y^i_t\}$.  
\begin{align*}
    H(Y_{\LocAgent[m,1:\numOfAgents]{1:T}}) &= H(\{y^1_T,y^2_T,...,y^{\numOfAgents'_T}_T\} |Y_{\LocAgent[m,1:\numOfAgents]{1:T-1}}) + H(Y_{\LocAgent[m,1:\numOfAgents]{1:T-1}}) \\
    &= \frac{1}{2} \log(det(2\pi e(\sigma^2 I + \kernel_{\LocAgent[m,1:\numOfAgents'_{T}]{T}}))) + H(\{y^1_{T-1},y^2_{T-1}....y^{\numOfAgents'_{T-1}}_{T-1} \}|Y_{\LocAgent[m,1:\numOfAgents]{1:T-2}}) + ... \\
    \tag{Since, $\{y^1_T,y^2_T,...,y^{\numOfAgents'_T}_T\}$  is jointly MV gaussian. $\sim \mathcal{|\Discat[i]|}\Big(\density_{T-1}(\LocAgent[m,1:\numOfAgents'_{T}]{T}), \sigma^2 I + \kernel_{\LocAgent[m,1:\numOfAgents'_{T}]{T}}\Big) $}\\
     &= \frac{1}{2} \numOfAgents'_{T} \log(2\pi e \sigma^2) +  \frac{1}{2} \log(det( I + \sigma^{-2} \kernel_{\LocAgent[m,1:\numOfAgents'_{T}]{T}})) + H(\{y^1_{T-1},y^2_{T-1}....y^{\numOfAgents'_{T-1}}_{T-1}\}|Y_{\LocAgent[m,1:\numOfAgents]{1:T-2}}) + ... \\ \tag{Since, $\frac{1}{2} \log(det(2\pi e(\sigma^2 I + \kernel_{\LocAgent[m,1:\numOfAgents'_{T}]{T}})))$ = $\frac{1}{2} \log({(2\pi e\sigma^2)}^{\numOfAgents'_{T}}det( I + \sigma^{-2}\kernel_{\LocAgent[m,1:\numOfAgents'_{T}]{T} }))$} \\
    &= \frac{1}{2} \sum_{t=1}^T \numOfAgents'_{t} \log(2\pi e \sigma^2) +  \frac{1}{2} \sum_{t=1}^T \log(det( I + \sigma^{-2} \kernel_{\LocAgent[m,1:\numOfAgents'_{t}]{t}}))  \tag{By recursively solving H(.|.) till t=1}\\
    H(Y_{\LocAgent[m,1:\numOfAgents]{1:T}}|\density) &= \frac{1}{2} \sum_{t=1}^T \numOfAgents'_{t} \log(2\pi e \sigma^2) \tag{entropy only because of noise} \\
     I(Y_{\LocAgent[m,1:\numOfAgents]{1:T}};\density) &= \frac{1}{2} \sum_{t=1}^T \log(det( I + \sigma^{-2} \kernel_{\LocAgent[m,1:\numOfAgents'_{t}]{t}})) 
\end{align*}
Using \eq~\ref{eqn: max-single-total-info}, Total information gain is given by:
\begin{align*}
    I(Y_{\LocAgent[m,1:\numOfAgents]{1:T}};\density) &= \frac{1}{2} \sum_{t=1}^T \log(det( I + \sigma^{-2} \kernel_{\LocAgent[m,1:\numOfAgents'_{t}]{t}})) \\
    &= \frac{1}{2} \sum_{t=1}^T \sum_{i=1}^{\numOfAgents'_{t}} \log( 1 + \sigma^{-2} \lambda_{i,t}) \numberthis \label{eqn: max-single-total-mutual-info-formulation}
\end{align*}

So far we have shown, $\actualRegret(T) \leq \sqrt{T \numOfAgents \frac{8\beta_t}{\log(1+|\Discat[i]|\sigma^{-2})}  \gamma_{\numOfAgents |\Discat[i]|T}}$, In this part we would like to bound $\gamma_{\numOfAgents |\Discat[i]|T}$. The analysis follow similar to \citep{gammaT-vakili21a} but for $\numOfAgents$ agents, each observing $|\Discat[i]_t|$ points at time $t$.
\begin{itemize}
    \item First we will decompose mutual information $I(Y_{\Discat[1:i]_{1:T}};\density)$ into "D-Dim" feature space (head) and the remaining feature dim (tail) \\
Using Mercer's theorem, a continuous p.d. kernel function can be written as,
\begin{align*}
    \funckernel (x,x') &= \sum_{m=1}^{\infty} \eigval_{m} \phi_m(x)\phi_m(x'),  \numberthis \label{eqn: mercer-eqn}
\end{align*}
where $\phi_m(x)$ are orthonormal eigen basis functions. A D dim feature space is given by $\varphi_D(.) = [\phi_1(.), \phi_2(.), \phi_3(.), ... \phi_D(.)]^{\trans}$. let $|\pfunckernel (x,x')| \leq \bar{\funckernel}$ and $|\phi_m(x)| \leq \bar{\phi} \ \forall x,x',m$. \\
Projection of $\density(.)$ to this D-dim space can be casted as,
\begin{align*}
    \mathcal{P}_D[\density(.)] = W^{\trans}_{D} \Lambda_D \varphi_D(.), 
\end{align*}
where $W^{\trans}_{D}$ is weight matrix. This can be thought as a sample from a dist. whose, associated covariance mat (kernel matrix) is $\pfunckernel (x,x') = \sum_{m=1}^{D} \eigval_{m} \phi_m(x)\phi_m(x')$. Hence,
\begin{align*}
   \funckernel (x,x')  &= \sum_{m=1}^{D} \eigval_{m} \phi_m(x)\phi_m(x') + \sum_{m=D + 1}^{\infty} \eigval_{m} \phi_m(x)\phi_m(x') \tag{decomposition of \eq~\ref{eqn: mercer-eqn}}\\
    &= \pfunckernel (x,x') + \ofunckernel (x,x') \numberthis \label{eqn: kernel-decomposition}
\end{align*}

\begin{align*}
    I(Y_{\Discat[1:i]_{1:T}};\density) &= \frac{1}{2} \sum_{t=1}^T \sum_{i=1}^\numOfAgents \sum_{p=1}^{|\Discat[i-]_t|} \log( 1 + \sigma^{-2} \lambda_p) \tag{from patch obs \todo{remove it}}\\
                 &= \frac{1}{2} \log( \det( I + \sigma^{-2} \kernel_{\Discat[1:i]_{1:T}})) \tag{$\kernel_{\Discat[1:i]_{1:T}}$ is a kernel matrix will all data points}\\
                 &= \frac{1}{2} \log( \det( I + \sigma^{-2} (\pkernel_{\Discat[1:i]_{1:T}} + \okernel_{\Discat[1:i]_{1:T}})) \tag{Using \eq~\ref{eqn: kernel-decomposition}}\\
                &= \frac{1}{2} \log \bigg( \det\Big( (I + \sigma^{-2} \pkernel_{\Discat[1:i]_{1:T}}) ( I + \sigma^{-2}(I + \sigma^{-2} \pkernel_{\Discat[1:i]_{1:T}})^{-1} \okernel_{\Discat[1:i]_{1:T}} \Big) \bigg) \\
                &= \frac{1}{2} \log \big( \det (I + \sigma^{-2} \pkernel_{\Discat[1:i]_{1:T}}) \big) +  \frac{1}{2} \log \big ( \det \big( I + \sigma^{-2}(I + \sigma^{-2} \pkernel_{\Discat[1:i]_{1:T}})^{-1} \okernel_{\Discat[1:i]_{1:T}} \big) \big) \label{eqn: mutual-info-decomposition} \numberthis
\end{align*}
\item Bound first term in \eq~\ref{eqn: mutual-info-decomposition}, $\frac{1}{2} \log \big( \det (I + \sigma^{-2} \pkernel_{\Discat[1:i]_{1:T}}) \big)$\\

\textbf{Some definitions and inequalities:} \\
$\phi(.)$ is eigen basis function, $\varphi_D(.) = [\phi_1(.), \phi_2(.), ... , \phi_D(.)]^{\trans}$ and $\Phi_{t,D} = [\varphi^{\trans}_D(x_1), \varphi^{\trans}_D(x_2), ... , \varphi^{\trans}_D(x_t)]^{\trans}$
\begin{align*}
    \kernel_{\Discat[1:i]_{1:T}} &= \Phi_{\numOfAgents |\Discat[i]|T, D} \Lambda_D \Phi_{\numOfAgents |\Discat[i]|T, D}^\trans \tag{$|\Discat[i]|$ in \numOfAgents $|\Discat[i]|$T is indicative of max points under disk} \\ \tag{ doesn't corresponds that every disk observes $|\Discat[i]|$ points}\\
    \gram_{\Discat[1:i]_{1:T}} &= \Lambda_D^{\frac{1}{2}} \Phi_{\numOfAgents |\Discat[i]|T, D}^\trans \Phi_{\numOfAgents |\Discat[i]|T, D} \Lambda_D^{\frac{1}{2}} \tag{Eigenbasis feature matrix (DxD) (! Gram Matrix)}
\end{align*}

\begin{align*}
     \det (I + \sigma^{-2} \pkernel_{\Discat[1:i]_{1:T}}) &= \det (I + \sigma^{-2} \Phi_{\numOfAgents |\Discat[i]|T, D} \Lambda_{D} \Phi_{\numOfAgents |\Discat[i]|T,D}^{\trans})\\
    &= \det (I + \sigma^{-2} \Lambda_{D}^{1/2} \Phi_{\numOfAgents |\Discat[i]|T, D}^{\trans}  \Phi_{\numOfAgents |\Discat[i]|T,D} \Lambda_{D}^{1/2})  \tag{Weinstein–Aronszajn identity} \\
    &= \det (I + \sigma^{-2} \gram_{\Discat[1:i]_{1:T}}) \numberthis \label{eqn: det-equality}\\
    \| \phi_{D}(x_p) \Lambda_{D}^{1/2} \|^{2}_2 &= \sum_{m=1}^{D} \eigval_m \phi^2_{m}(x) \\
    &= \pfunckernel(x,x)\\
    &\leq \bar{\funckernel}  \numberthis \label{eqn: kernel-bound} \\
\textbf{Now consider},\\
   \trace (I + \sigma^{-2} \gram_{\Discat[1:i]_{1:t}})
    &= \trace \big( I + \sigma^{-2} \Lambda_{D}^{1/2} \Phi_{\numOfAgents |\Discat[i]|T, D}^{\trans}  \Phi_{\numOfAgents |\Discat[i]|T,D} \Lambda_{D}^{1/2} \big) \tag{From definition of $\gram_{\Discat[1:i]_{1:t}}$}\\
    &= D + \sigma^{-2} \trace \big( \Lambda_{D}^{1/2} \Phi_{\numOfAgents |\Discat[i]|T, D}^{\trans}  \Phi_{\numOfAgents |\Discat[i]|T,D} \Lambda_{D}^{1/2} \big) \\
    &= D + \sigma^{-2} \sum_{t=1}^t \sum_{i=1}^\numOfAgents \sum_{p=1}^{|\Discat[i-]_t|} \trace \big( \Lambda_{D}^{1/2} \varphi_{D}(x_p)^{\trans}  \varphi_{D}(x_p) \Lambda_{D}^{1/2} \big) \tag{Think as element wise (x) multiplication of $\numOfAgents |\Discat[i]|T$ with itself}\\
    &= D + \sigma^{-2} \sum_{t=1}^t \sum_{i=1}^\numOfAgents \sum_{p=1}^{|\Discat[i-]_t|} \| \phi_{D}(x_p) \Lambda_{D}^{1/2} \|^{2}_2 \\ 
    &\leq D + \sigma^{-2} \sum_{t=1}^t \sum_{i=1}^\numOfAgents |\Discat[i-]_t| \bar{\funckernel} \tag{$\sum_{p=1}^{|\Discat[i-]_t|} 1 = |\Discat[i-]_t|$ and using \eq~\ref{eqn: kernel-bound}}\\
    &\leq D + \sigma^{-2} t \numOfAgents |\Discat[i]| \bar{\funckernel} \numberthis \label{eqn: trace-kernel-p}\\
\textbf{Now consider},\\
\log \big( \det (I + \sigma^{-2} \pkernel_{\Discat[1:i]_{1:t}}) \big) &= \log \big( \det (I + \sigma^{-2} \gram_{\Discat[1:i]_{1:T}}) \big) \tag{Using \eq~\ref{eqn: det-equality}}\\
&\leq D \log \Big( \frac{\trace (I + \sigma^{-2} \gram_{\Discat[1:i]_{1:T}})}{D} \Big)\tag{$\log(\det (A_n)) \leq n \log(\frac{\trace(A_n)}{n})$}\\
&\leq D \log \Big( \frac{D + \sigma^{-2} t \numOfAgents |\Discat[i]| \bar{\funckernel}}{D} \Big) \tag{Using \eq~\ref{eqn: trace-kernel-p}} \\
&= D \log \Big( 1 + \frac{\sigma^{-2} t \numOfAgents |\Discat[i]| \bar{\funckernel}}{D} \Big) \numberthis \label{eqn: bound-log-det-kernelp} 
\end{align*}
\item Bound $2^{nd}$ term, $\frac{1}{2} \log \big ( \det \big( I + (I + \sigma^{-2} \pkernel_{\Discat[1:i]_{1:T}})^{-1} \okernel_{\Discat[1:i]_{1:T}} \big) \big)$, \\

Using the upper bound of eigen basis function i.e., $|\phi_m(x) \leq \bar{\phi}|$, define $\delta_D$,
\begin{align*}
    \delta_{D} \coloneqq \sum_{m= D+1}^\infty \lambda_m \bar{\phi}.
\end{align*} 
Since, $\ofunckernel(x,x') \leq \delta_{D}$ 
\begin{align*}
\implies \trace ( \okernel_{\Discat[1:i]_{1:T}} ) \leq \delta_D \sum_{t=1}^t \sum_{i=1}^\numOfAgents \sum_{p=1}^{\Discat[1:i]_{1:T}} 1 \leq KNt\delta_D \numberthis \label{eqn: trace-kernel-o-bound}
\end{align*}
Let's consider, 
\begin{align*}
    \trace \big((I + \sigma^{-2} \pkernel_{\Discat[1:i]_{1:T}})^{-1} \okernel_{\Discat[1:i]_{1:T}} \big) &\leq \trace ( \okernel_{\Discat[1:i]_{1:T}} ) \tag{min $\eigval$ of ($I + \sigma^{-2} \pkernel_{\Discat[1:i]_{1:T}}) \geq 1$  }\\
    &\leq KNt \delta_D \tag{Using \eq~\ref{eqn: trace-kernel-o-bound}} \\
    \implies    \trace \big(I + \sigma^{-2}(I + \sigma^{-2} \pkernel_{\Discat[1:i]_{1:T}})^{-1} \okernel_{\Discat[1:i]_{1:T}} \big) &\leq \trace ( I + \sigma^{-2}\okernel_{\Discat[1:i]_{1:T}} ) \\
    &\leq KNt (1+\sigma^{-2}\delta_D) \\
\log \Big( \det \big(I + \sigma^{-2}(I + \sigma^{-2} \pkernel_{\Discat[1:i]_{1:T}})^{-1} \okernel_{\Discat[1:i]_{1:T}} \big) \Big) &\leq KNt \log (1 + \sigma^{-2} \delta_D ) \tag{Since, $\log(\det (A_n)) \leq n \log(\frac{\trace(A_n)}{n})$} \\ 
        & \leq \sigma^{-2} KNt  \delta_D \tag{Using $\log (1+x) \leq x$}
\end{align*}
Inserting this inequality along with \eq~\ref{eqn: bound-log-det-kernelp} in \eq~\ref{eqn: mutual-info-decomposition}, we get,
\begin{align*}
I(Y_{\Discat[1:i]_{1:T}};\density)
                &= \frac{1}{2} \log \big( \det (I + \sigma^{-2} \pkernel_{\Discat[1:i]_{1:T}}) \big) +  \frac{1}{2} \log \big ( \det \big( I + \sigma^{-2}(I + \sigma^{-2} \pkernel_{\Discat[1:i]_{1:T}})^{-1} \okernel_{\Discat[1:i]_{1:T}} \big) \big) \\
                &\leq \frac{1}{2} D \log \Big( 1 + \frac{\sigma^{-2} t \numOfAgents |\Discat[i]| \bar{\funckernel}}{D} \Big) +  \frac{1}{2} \sigma^{-2} KNt  \delta_D \\
    \gamma_{\numOfAgents |\Discat[i]|T} &= sup_{x_T \subseteq V} I(Y_{\Discat[1:i]_{1:T}};\density) \\
    & \leq \frac{1}{2} D \log \Big( 1 + \frac{\sigma^{-2} t \numOfAgents |\Discat[i]| \bar{\funckernel}}{D} \Big) +  \frac{1}{2} \sigma^{-2} KNt  \delta_D \numberthis \label{eqn: bound-mutual-info-D}
\end{align*}
\item Now, we will try to bound \eq~\ref{eqn: bound-mutual-info-D}, by picking up suitable $D$.

\begin{enumerate}
    \item Assuming polynomial eigen decay
    \begin{align*}
        \delta_D &= \sum_{m = D+1}^{\infty} \eigval_m \bar{\phi}^2 \\
        &\leq \sum_{m = D+1}^{\infty} \polyCoeff m^{-\polyExponent} \bar{\phi}^2 \\
        &\leq \int_{z = D}^{\infty} \polyCoeff z^{-\polyExponent} \bar{\phi}^2 dz \\
        &=\polyCoeff D^{1-\polyExponent} \bar{\phi}^2 \tag{$ \frac{\polyCoeff}{\polyExponent-1} D^{1-\polyExponent} \bar{\phi}^2$}
    \end{align*}
if we pick $D = \lceil (\polyCoeff \bar{\phi}^2 \numOfAgents |\Discat[i]|T)^{\frac{1}{\polyExponent}} 
\sigma^{\frac{-2}{\polyExponent}} \log^{\frac{-1}{\polyExponent}} ( 1 + \sigma^{-2} t \numOfAgents |\Discat[i]| \bar{\funckernel})\rceil$, which is the smallest $D$ ensuring $\sigma^{-2} \numOfAgents |\Discat[i]|T \delta_D \leq D \log (1 + \sigma^{-2}  \numOfAgents |\Discat[i]| T \bar{\funckernel})$

Using this $D$, from \eq~\ref{eqn: bound-mutual-info-D}, we get bound on $\gamma_{\numOfAgents |\Discat[i]|T}$ as,

\begin{align*}
    \gamma_{\numOfAgents |\Discat[i]|T} \leq \Big( (\polyCoeff \bar{\phi}^2 \numOfAgents |\Discat[i]|T)^{\frac{1}{\polyExponent}} 
\sigma^{\frac{-2}{\polyExponent}} \log^{\frac{-1}{\polyExponent}} ( 1 + \sigma^{-2} \numOfAgents |\Discat[i]| T \bar{\funckernel}) + 1 \Big) \log( 1 + \sigma^{-2}  \numOfAgents |\Discat[i]| T \bar{\funckernel})
\end{align*}

This implies, 
\begin{align*}
    \actualRegret \leq \sqrt{T \numOfAgents \frac{8\beta_t}{\log(1+|\Discat[i]|\sigma^{-2})}  \Big( (\polyCoeff \bar{\phi}^2 \numOfAgents |\Discat[i]|T)^{\frac{1}{\polyExponent}}
\sigma^{\frac{-2}{\polyExponent}} \log^{\frac{-1}{\polyExponent}} ( 1 + \sigma^{-2} \numOfAgents |\Discat[i]| T \bar{\funckernel}) + 1 \Big) \log( 1 + \sigma^{-2}  \numOfAgents |\Discat[i]| T \bar{\funckernel})}
\end{align*}
$\actualRegret = \mathcal{O} \big( (\numOfAgents |\Discat[i]|T)^{\frac{\polyExponent + 1}{2 \polyExponent}} \log^{\frac{\polyExponent - 1}{2 \polyExponent}}( \numOfAgents  T ) \log^{ 1/2 - \frac{1}{\polyExponent}}(  |\Discat[i]|  ) \big)$

\item Assuming exponential eigen decay
    \begin{align*}
        \delta_D &= \sum_{m = D+1}^{\infty} \eigval_m \bar{\phi}^2 \\
        &\leq \sum_{m = D + 1 }^{\infty} \expCoeff \exp (- \expExponentCoeff m^{\expExponentExponent}) \bar{\phi}^2 \\
        &\leq \int_{z = D}^{\infty} \expCoeff \exp (- \expExponentCoeff z^{\expExponentExponent}) \bar{\phi}^2 dz 
    \end{align*}
There are two possible cases here, \\
\textbf{Part i)} $\expExponentExponent = 1$, \\
\begin{align*}
    \int_{z = D}^{\infty} \expCoeff \exp (- \expExponentCoeff z^{\expExponentExponent}) \bar{\phi}^2 dz &= 
    \int_{z = D}^{\infty} \expCoeff \exp (- \expExponentCoeff z) \bar{\phi}^2 dz \\
    &= \frac{\expCoeff \bar{\phi}^2}{\expExponentCoeff} \exp (-\expExponentCoeff D)
\end{align*}
if we pick $D = \lceil \frac{1}{\expExponentCoeff} \log (\frac{\expCoeff \bar{\phi}^2 \numOfAgents |\Discat[i]|T \sigma^{-2}}{\expExponentCoeff}) \rceil$, which is the smallest $D$ ensuring $\sigma^{-2} \numOfAgents |\Discat[i]|T \delta_D \leq D \log (1 + \sigma^{-2}  \numOfAgents |\Discat[i]| T \bar{\funckernel})$ (Actually with this $D$, the LHS of inequality is $\leq$ 1) (also, $D = \lceil \frac{2}{\expExponentCoeff} \log (\frac{\expCoeff \bar{\phi}^2 \numOfAgents |\Discat[i]|T \sigma^{-2}}{\expExponentCoeff}) \rceil $is used finally)

\textbf{Part ii)} $\expExponentExponent \neq 1$, \\
\begin{align*}
    \int_{z = D}^{\infty} \expCoeff \exp (- \expExponentCoeff z^{\expExponentExponent}) \bar{\phi}^2 dz &= 
    \frac{1}{\expExponentExponent} \int_{y = D^{\expExponentExponent}}^{\infty} y^{\frac{1}{\expExponentExponent} - 1 }\expCoeff \exp (- \expExponentCoeff y) \bar{\phi}^2 dy \\
    &= 
    \frac{\expCoeff}{\expExponentExponent} \int_{y = D^{\expExponentExponent}}^{\infty} y^{\frac{1}{\expExponentExponent} - 1 }\expCoeff \exp (- \expExponentCoeff \frac{y}{2}) \exp (- \expExponentCoeff \frac{y}{2})  \bar{\phi}^2 dy \\
    &\leq 
    \frac{\expCoeff}{\expExponentExponent} \int_{y = D^{\expExponentExponent}}^{\infty} \Big( \frac{2}{\expExponentCoeff} \big( \frac{1}{\expExponentExponent} - 1 \big) \Big)^{\frac{1}{\expExponentExponent} - 1} \exp (- ( \frac{1}{\expExponentExponent} - 1 ) ) \exp (- \expExponentCoeff \frac{y}{2})  \bar{\phi}^2 dy \\
    &=  
    \frac{2 \expCoeff}{\expExponentCoeff \expExponentExponent } \Big( \frac{2}{\expExponentCoeff} \big( \frac{1}{\expExponentExponent} - 1 \big) \Big)^{\frac{1}{\expExponentExponent} - 1} \exp (- ( \frac{1}{\expExponentExponent} - 1 ) ) \exp (- \expExponentCoeff \frac{D^\expExponentExponent}{2})  \bar{\phi}^2
\end{align*}
if we pick 
\begin{align*}
    D = \Bigg\lceil  \bigg(\frac{2}{\expExponentCoeff} \Big( \log(\numOfAgents |\Discat[i]|T) + \log\big( 
    \frac{2 \expCoeff \bar{\phi}^2 \sigma^{-2}}{\expExponentCoeff \expExponentExponent } \big) + 
    (\frac{1}{\expExponentExponent} - 1) 
    \Big( \log \Big( \frac{2}{\expExponentCoeff} \big( \frac{1}{\expExponentExponent} - 1 \big)\Big) -1 \Big) 
    \Big) \bigg)^{\frac{1}{\expExponentExponent}} \Bigg\rceil
\end{align*}
which is the smallest $D$ ensuring $\sigma^{-2} \numOfAgents |\Discat[i]|T \delta_D \leq D \log (1 + \sigma^{-2}  \numOfAgents |\Discat[i]| T \bar{\funckernel})$ (Actually with this $D$, the LHS of inequality is $\leq$ 1)\\

\textbf{Combining both the cases:} \\
Using this $D$, from \eq~\ref{eqn: bound-mutual-info-D}, we get bound on $\gamma_{\numOfAgents |\Discat[i]|T}$ as,

\begin{align*}
    \gamma_{\numOfAgents |\Discat[i]|T} \leq  \bigg( \Big(\frac{2}{\expExponentCoeff} \big( \log(\numOfAgents |\Discat[i]|T) + C_{\expExponentExponent} 
    \big) \Big)^{\frac{1}{\expExponentExponent}} + 1 \bigg) \log( 1 + \sigma^{-2}  \numOfAgents |\Discat[i]| T \bar{\funckernel})
\end{align*}
where, $C_{\expExponentExponent} = \log\big( 
    \frac{2 \expCoeff \bar{\phi}^2 \sigma^{-2}}{\expExponentCoeff \expExponentExponent } \big) + 
    (\frac{1}{\expExponentExponent} - 1) 
    \Big( \log \big( \frac{2}{\expExponentCoeff} \big( \frac{1}{\expExponentExponent} - 1 \big) \big) -1 \Big)$ when $\expExponentExponent \neq 1 $, and $C_{\expExponentExponent} = \log\big( 
    \frac{\expCoeff \bar{\phi}^2 \sigma^{-2}}{\expExponentCoeff} \big)$ when $\expExponentExponent = 1$.\\
This implies, 
\begin{align*}
    \actualRegret &\leq \sqrt{T \numOfAgents \frac{8\beta_t}{\log(1+|\Discat[i]|\sigma^{-2})}  \bigg( \Big(\frac{2}{\expExponentCoeff} \big( \log(\numOfAgents |\Discat[i]|T) + C_{\expExponentExponent} 
    \big) \Big)^{\frac{1}{\expExponentExponent}} + 1 \bigg) \log( 1 + \sigma^{-2}  \numOfAgents |\Discat[i]| T \bar{\funckernel})}\\
\actualRegret &= \mathcal{O} \big( (KT)^{\frac{1}{2}} \log^{1 + \frac{1}{\expExponentExponent}}( \numOfAgents T ) \log^{\frac{1}{\expExponentExponent}}(|\Discat[i]|) \big)
\end{align*}

\end{enumerate}

% \begin{align*}
%     \log \det (P) \leq n \log(\trace(P)/n)
% \end{align*}

\end{itemize}
